# Supplementary material for: Exchange-of-Thought: Enhancing Large Language Model Capabilities through Cross-Model Communication
Source: arXiv:2312.01823 source file (2023-12-04)
Supplement: Supplementary file 2 [file baselines.tex]

\section{Baselines}
\label{appendix:app-baselines}
